# Supplementary material for: Humanoid Parkour Learning
Source: arXiv:2406.10759 source file (2024-09-26)
Supplement: Supplementary file 1 [file supp-example.tex]

\documentclass{article}

\usepackage{corl_2024} % Use this for the initial submission.
%\usepackage[final]{corl_2024} % Uncomment for the camera-ready ``final'' version.
% \usepackage[preprint]{corl_2024} % Uncomment for pre-prints (e.g., arxiv); This is like ``final'', but will remove the CORL footnote.

\usepackage{graphics,graphicx,float,subcaption,booktabs,xcolor,multirow,array,color,ifthen,tabu,colortbl,dblfloatfix,url,xparse,mathtools,patchcmd,amssymb,xspace,nicefrac,microtype,amsmath,amsthm,amsfonts,bm,ragged2e,tikz,stackengine,etoolbox,xpatch,enumerate,xstring,setspace,tabularx,makecell,changepage,cuted,titlesec,enumitem,wrapfig,tcolorbox,gensymb,algorithm,algpseudocode,makecell,bbm}

\title{Supplementary Material: \\ Humanoid Parkour Learning}

% The \author macro works with any number of authors. There are two
% commands used to separate the names and addresses of multiple
% authors: \And and \AND.
%
% Using \And between authors leaves it to LaTeX to determine where to
% break the lines. Using \AND forces a line break at that point. So,
% if LaTeX puts 3 of 4 authors names on the first line, and the last
% on the second line, try using \AND instead of \And before the third
% author name.

% NOTE: authors will be visible only in the camera-ready and preprint versions (i.e., when using the option 'final' or 'preprint'). 
% 	For the initial submission the authors will be anonymized.

\author{
Ziwen Zhuang\textsuperscript{12}, Shenzhe Yao\textsuperscript{12}, Hang Zhao\textsuperscript{13}\\
\textsuperscript{1}Shanghai Qi Zhi, \textsuperscript{2}ShanghaiTech, \textsuperscript{3}Tsinghua\\
}


\begin{document}

\makeatletter
\let\@oldmaketitle\@maketitle%
\renewcommand{\@maketitle}{\@oldmaketitle%
\centering
\bigskip}
\makeatother
\maketitle

\appendix
\input{supp}
\bibliography{example}

\end{document}
